# Supplementary material for: The Ingleton inequality holds for metacyclic groups and fails for supersoluble groups
Source: arXiv:2505.22565 ancillary file (2025-05-28)
Supplement: Supplementary file 1 [file ingleton.pdf]

# Magma Package **ingleton**

David A. Craven

Version 1.0: April 8, 2025

# Contents

|     |                               |   |
|-----|-------------------------------|---|
| 0.1 | Accessing databases . . . . . | 1 |
| 0.2 | Computing violators . . . . . | 1 |
| 0.3 | Computing offenders . . . . . | 2 |

The aim of this documentation is to cover all of the new commands introduced in the `ingleton` package. To run it, use `AttachSpec("ingleton.s");`.

## 0.1 Accessing databases

`AllIngletonViolators() -> SeqEnum`

Returns all Ingleton violators  $G$  of order at most 1023. There are returned as a list, in the form  $\langle n, i \rangle$ , where  $G$  is `SmallGroup(n,i)` in the `SmallGroup` database.

`AllIrreducibleIngletonViolators() -> SeqEnum`

Returns all irreducible Ingleton violators  $G$  of order at most 1023. There are returned as a list, in the form  $\langle n, i \rangle$ , where  $G$  is `SmallGroup(n,i)` in the `SmallGroup` database.

`AllIndomitableIngletonViolators() -> SeqEnum`

Returns all indomitable Ingleton violators  $G$  of order at most 1023. There are returned as a list, in the form  $\langle n, i \rangle$ , where  $G$  is `SmallGroup(n,i)` in the `SmallGroup` database.

`IrreducibleIngletonOffenderDatabase() -> SeqEnum`

Returns representatives from all conjugacy classes of irreducible Ingleton offenders in groups of order up to 720, and currently one group of order 768. The output is a sequence of 4-tuples, each entry containing the group, a sequence of subgroups  $H_i$ , the Ingleton ratio and the Ingleton score.

`IndomitableIngletonOffenderDatabase() -> SeqEnum`

Returns representatives from all conjugacy classes of indomitable Ingleton offenders in groups of order up to 720, and currently one group of order 768. The output is a sequence of 4-tuples, each entry containing the group, a sequence of subgroups  $H_i$ , the Ingleton ratio and the Ingleton score.

## 0.2 Computing violators

`IsIrreducibleIngletonViolatorMinimal(G::Grp:Verbosity:=false,DoneSoFar:=0) -> Bool,SeqEnum`

Returns true if  $G$  is an irreducible Ingleton violator in a minimal sense. This is faster than the General algorithm, and if it returns true then the group is an Ingleton violator, but if there is a proper subgroup that is also an Ingleton violator it might return false and the group still be an irreducible Ingleton violator. Use parameter `Verbosity` to give some commentary, and `DoneSoFar:=n` if you want to start from subgroup  $n+1$  (for example, if you have previously terminated a running program, or are parallelizing it to save time).

Warning: if you give  $G$  in two different forms, for example as a PC group and then as a permutation group, or as two different permutation groups, the ordering on the groups will probably be different, and the `DoneSoFar` parameter should be used with great care.

`IsIrreducibleIngletonViolatorGeneral(G::Grp:Verbosity:=false,DoneSoFar:=0) -> Bool,SeqEnum`

Returns true if  $G$  is an irreducible Ingleton violator. This is much slower than the Minimal algorithm, but guarantees the correct result. The recommendation is to run the Minimal algorithm first unless you believe that  $G$  is not an irreducible Ingleton violator. Use parameter `Verbosity` to give some commentary,

and `DoneSoFar:=n` if you want to start from subgroup `n+1` (for example, if you have previously terminated a running program, or are parallelizing it to save time).

Warning: if you give `G` in two different forms, for example as a PC group and then as a permutation group, or as two different permutation groups, the ordering on the groups will probably be different, and the `DoneSoFar` parameter should be used with great care.

`IsIndomitableIngletonViolatorMinimal(G::Grp:Verbosity:=false,DoneSoFar:=0) -> Bool,SeqEnum`

Returns true if `G` is an indomitable Ingleton violator in a minimal sense. This is faster than the General algorithm, and if it returns true then the group is an Ingleton violator, but if there is a proper subgroup that is also an Ingleton violator it might return false and the group still be an indomitable Ingleton violator. Use parameter `Verbosity` to give some commentary, and `DoneSoFar:=n` if you want to start from subgroup `n+1` (for example, if you have previously terminated a running program, or are parallelizing it to save time).

Warning: if you give `G` in two different forms, for example as a PC group and then as a permutation group, or as two different permutation groups, the ordering on the groups will probably be different, and the `DoneSoFar` parameter should be used with great care.

`IsIndomitableIngletonViolatorGeneral(G::Grp:Verbosity:=false,DoneSoFar:=0) -> Bool,SeqEnum`

Returns true if `G` is an indomitable Ingleton violator. This is much slower than the Minimal algorithm, but guarantees the correct result. The recommendation is to run the Minimal algorithm first unless you believe that `G` is not an indomitable Ingleton violator. Use parameter `Verbosity` to give some commentary, and `DoneSoFar:=n` if you want to start from subgroup `n+1` (for example, if you have previously terminated a running program, or are parallelizing it to save time).

Warning: if you give `G` in two different forms, for example as a PC group and then as a permutation group, or as two different permutation groups, the ordering on the groups will probably be different, and the `DoneSoFar` parameter should be used with great care.

### 0.3 Computing offenders

`ListIngletonOffendersMinimal(G::Grp:Verbosity:=false,DoneSoFar:=0) -> SeqEnum,SeqEnum`

Returns a list of all irreducible and indomitable Ingleton offenders respectively. The offenders are returned as a 4-tuple: the group `G`, the subgroups `H1`, `H2`, `H3`, `H4`, the Ingleton ratio of the offender and the Ingleton score of the offender. This will only return all offenders if `G` is a minimal Ingleton violator, but is much faster than the General algorithm. Use parameter `Verbosity` to give some commentary, and `DoneSoFar:=n` if you want to start from subgroup `n+1` (for example, if you have previously terminated a running program, or are parallelizing it to save time).

Warning: if you give `G` in two different forms, for example as a PC group and then as a permutation group, or as two different permutation groups, the ordering on the groups will probably be different, and the `DoneSoFar` parameter should be used with great care.

`ListIngletonOffendersGeneral(G::Grp:Verbosity:=false,DoneSoFar:=0) -> SeqEnum,SeqEnum`

Returns a list of all irreducible and indomitable Ingleton offenders respectively. The offenders are returned as a 4-tuple: the group `G`, the subgroups `H1`, `H2`, `H3`, `H4`, the Ingleton ratio of the offender and the Ingleton score of the offender. This will return all offenders, but will be slower than the Minimal algorithm, that can

only be used when there is no proper subgroup that is also an Ingleton violator. Use parameter **Verbosity** to give some commentary, and **DoneSoFar:=n** if you want to start from subgroup **n+1** (for example, if you have previously terminated a running program, or are parallelizing it to save time).

Warning: if you give **G** in two different forms, for example as a PC group and then as a permutation group, or as two different permutation groups, the ordering on the groups will probably be different, and the **DoneSoFar** parameter should be used with great care.
